# Supplementary material for: Mean-Field Approximation to Gaussian-Softmax Integral with Application to Uncertainty Estimation
Source: arXiv:2006.07584 source file (2021-05-09)
Supplement: Supplementary file 1 [file appendix_mf.tex]

%!TEX root = main_jmlr2021.tex
\section{Mean-Field Approximation for Gaussian-softmax Integration}\label{sMFDerivation}
In this section, we derive the mean-field approximation for Gaussian-softmax integration, eq.~(\ref{eGaussianSoftmax}) in the main text. Assume the same notations as in \S\ref{sMF}, where the activation to softmax follows a Gaussian $\va \sim \sN(\vmu, \mS)$.
\begin{align}
e_k  & = \expect{}{f_k} = \int \textsc{softmax}(a_k) \sN(\va; \vmu, \mS) \mathrm{d}\va \notag \\
 & = \int \frac{1}{1 + \sum_{i \ne k} e ^{- (a_k - a_{i})} } \sN(\va; \vmu, \mS) \mathrm{d}\va
 \notag \\
& = \int \left( 2 -K + \sum_{i \ne k}\frac{1}{\sigma(a_k - a_{i})} \right)^{-1} \sN(\va; \vmu, \mS) \mathrm{d}\va 
 \notag \\
&  \mathrel{\substack{\text{integrate}\\\approx\\\text{independently}}}   \left(2 -K + \sum_{i \ne k}\frac{1}{\expect{p(a_i, a_k)}{\sigma (a_k - a_i)}}\right)^{-1}   \label{eSepInt}
\end{align}
where ``integrate independently'' means integrating each term in the summand independently, resulting the expectation to the marginal  distribution over the pair $(a_i, a_k)$. This approximation is prompted by the mean-field approximation: $\expect{}{f(x)} \approx f(\expect{}{x})$ for a nonlinear function $f(\cdot)$\footnote{Similar to the classical use of mean-field approximation on Ising models, we use the term mean-field approximation to capture the notion that the expectation is  computed by considering the weak, pairwise coupling effect from points on the lattice, \ie,  $a_i$ with $i\ne k$.}.

Next we plug in the approximation to $\expect{}{\sigma(\cdot)}$ where $\sigma(\cdot)$ is the sigmoid function, which states that
\begin{equation}
\int \sigma(x) N(x; \mu, s^2) \mathrm{d}x \approx \sigma\left(\frac{\mu}{\sqrt{1+\lambda_0 s^2}}\right).\label{eqn:eSigmoid}
\end{equation}
$\lambda_0$ is a constant and is usually chosen to be $\pi/8$ or $3/\pi^2$.  This is a well-known result, see~\cite{bishop06}. 
We further approximate by considering different ways to compute the bivariate expectations in the denominator.

\paragraph{Mean-Field 0 ($\cst{mf0}$)}   In the denominator, we ignore the variance of $a_i$ for $i\ne k$ and replace $a_i$ with its mean $\mu_i$, and compute the expectation only with respect to $\alpha_k$. We arrive at
\begin{equation*} 
e_k \approx  \left(2 -K + \sum_{i \ne k}\frac{1}{\expect{p(a_k)}{\sigma (a_k - \mu_i)}}\right)^{-1}.
\end{equation*} 
Applying eq.(\ref{eqn:eSigmoid}), we have
\begin{equation}
e_k \approx \left( 2-K + \sum_{i\ne k }\frac{1}{
\sigma\left( \frac{\mu_k - \mu_{i}}{\sqrt{1+ \lambda_0 s_k^2}}      \right)} \right)^{-1}
= \left( \sum_{i} \exp \left(- \frac{\mu_k - \mu_{i}}{\sqrt{1+ \lambda_0 s_k^2 }}\right) \right)^{-1}.
\end{equation}

\paragraph{Mean-Field 1 ($\cst{mf1}$)} If we replace $p(a_i, a_k)$ with the two independent marginals $p(a_i)p(a_k)$ in the denominator, recognizing $(a_k - a_i) \sim \sN(\mu_k-\mu_i, s_i^2+s_k^2)$, we get,
\begin{equation}
e_k \approx \left( 2-K + \sum_{i\ne k }\frac{1}{
\sigma\left( \frac{\mu_k - \mu_{i}}{\sqrt{1+ \lambda_0 (s_i^2 + s_k^2)}}     \right)} \right)^{-1} 
\!\! = \left( \sum_{i} \exp \left(- \frac{\mu_k - \mu_{i}}{\sqrt{1+ \lambda_0 (s_k^2 + s_i^2)}}\right) \right)^{-1}.
\label{eqn:eMFIndependent}
\end{equation}

\paragraph{Mean-Field 2 ($\cst{mf2}$)} Lastly, if we compute eq.(\ref{eSepInt}) with a full covariance between $a_i$ and $a_k$, recognizing $(a_k - a_i) \sim \sN(\mu_k-\mu_i, s_i^2+s_k^2-2s_{ik})$, we get
\begin{align}
e_k  \approx & \left( 2-K  + \sum_{i\ne k }\frac{1}{
\sigma\left( \frac{\mu_k - \mu_{i}}{\sqrt{1+ \lambda_0 (s_i^2 + s_k^2 - 2s_{ik})}}      \right)} \right)^{-1} \notag \\
& = \left( \sum_{i} \exp \left(- \frac{\mu_k - \mu_{i}}{\sqrt{1+ \lambda_0 (s_k^2 + s_i^2-2s_{ik})}}\right) \right)^{-1}.
\label{eqn:eMFfull}
\end{align}
We note that ~\cite{daunizeau2017semi} has developed the approximation form eq.(\ref{eqn:eMFfull}) for computing $e_k$, though the author did not use it for uncertainty estimation.
